# Supplementary material for: CNN with large memory layers
Source: arXiv:2101.11685 source file (2021-04-26)
Supplement: Supplementary file 1 [file appendix.tex]

\chapter*{Appendix}

proofs, extra figures, etc.
